# Supplementary material for: Robots of the Lost Arc: Self-Supervised Learning to Dynamically Manipulate Fixed-Endpoint Cables
Source: arXiv:2011.04840 source file (2024-05-02)
Supplement: Supplementary file 1 [file section-8-appendix.tex]

\normalsize
% \onecolumn
% \appendix
\section{Appendix}
\label{sec:appendix}
The appendix is organized as follows:

\daniel{TODO insert extra text here}
